# Supplementary material for: Linear Dynamics: Clustering without identification
Source: arXiv:1908.01039 source file (2020-02-29)
Supplement: Supplementary file 1 [file appendix_ar_dist_to_eig_dist.tex]

\section{Correlation between AR parameter distance and LDS eigenvalue distance}\label{sec:ar_dist_to_eig_dist}

In Theorem \ref{thm:approx_eig}, we show that small distance between autoregressive parameters guarantees small distance between the eigenvalues of corresponding LDSs. Here we show the converse is also true, i.e. the autoregressive cofficients are similar when the dynamical systems are similar.

\begin{lemma}
Let $A$ and $A'$ be two real-valued matrices with characteristic polynomials $u^n + \varphi_1 u^{n-1} + \cdots + \varphi_{n-1}u + \varphi_n,$ and $u^n + \varphi_1' u^{n-1} + \cdots + \varphi_{n-1}'u + \varphi_n'.$ Then $$|\varphi_k'-\varphi_k| \leq (n-k+1) |\varphi_{k-1}|\  \norm{ A-A'}_2 + \mathcal{O}(\norm{ A-A'}_2^2),$$ where $\varphi_0$ is taken to be 1.
\end{lemma}
\begin{proof}
See~\cite{ipsen2008perturbation}.
\end{proof}

The $\ell_2$ polynomial norm of a polynomial $\Phi(u) = u^n + \varphi_1 u^{n-1} + \cdots + \varphi_{n-1}u + \varphi_n$ is defined as
$$\norm{\Phi}_2 = \sqrt{\sum_{k=0}^n |\varphi_k|^2}.$$

\begin{corollary}
Let $X = (S, A, b, \sigma_{\epsilon}, M)$ and $X' = (S, A', b', \sigma'_{\epsilon}, M')$ be two LDSs as defined above. Let $\varphi_0 (= 1), \varphi_1, \varphi_2, \cdots, \varphi_n$ be the autoregressive coefficients in any measurement series $y^j(t)$, and let $\varphi'_0 (= 1), \varphi'_1, \varphi'_2, \cdots, \varphi'_n$ be the autoregressive coefficients in any measurement series $y'^{j'}(t)$. Then, 
$$\norm{\Phi - \Phi'}_2 \leq n \norm{A-A'}_2 \norm{\Phi}_2 + \mathcal{O}(\norm{A-A'}_2^2).$$
\end{corollary}

Note that since the autoregressive coefficients are invariant under change of basis of $A$, the above still holds if $\norm{A-A'}_2$ is replaced by $\min_{V}\norm{VAV^T-A'}_2$ over all change of basis matrix $V$.
